# Supplementary material for: Unpaired cross-modality educed distillation (CMEDL) for medical image segmentation
Source: arXiv:2107.07985 source file (2021-12-07)
Supplement: Supplementary file 1 [file Supplementary.pdf]

# Supplementary Document: Unpaired cross-modality educed distillation (CMEDL) for medical image segmentation

## I. DATASET DETAILS

### A. CT dataset

We analyzed non-small cell lung cancer (NSCLC) patient datasets obtained from both internal archive and the open source NSCLC-TCIA dataset, both consisting of patients diagnosed with lung cancers and imaged with CT prior to radiation treatment. Patient images were acquired predominantly using Siemens (N=281), while the rest used CMS Inc (N = 96) for the open-source NSCLC-TCIA, while all of the internal validation and testing datasets were acquired on the GE scanners. All patients were biopsy confirmed to have stage II to III lung cancers and underwent treatment with definitive radiotherapy and the internal patients were also treated with immunotherapy. The TCIA dataset was acquired predominantly with an image resolution of 0.98mm×0.98mm×3mm. The validation dataset consisted of 209 tumors arising from 50 patients and the testing dataset consisted of 609 tumors arising from 177 lung cancer patients treated with immunotherapy following chemoradiotherapy from internal archive dataset. The internal dataset was acquired with a predominant image resolution of 0.67mm×0.67mm×5mm. Contrast and non-contrast CT scans with both lung and standard reconstruction kernels as well as smooth and sharper reconstructions were analyzed. However, no thin scans were (that is below 3mm) were analyzed.

### B. MRI lung tumor dataset

A total of 82 T2-weighted (T2W) MRIs from 28 patients enrolled in a prospective IRB-approved study with non-small lung cancer (NSCLC) scanned on a 3T Philips Ingenia scanner (Medical Systems, Best, Netherlands) before and every week during conventional fractionated external beam radiotherapy of 60 Gy were analyzed. Nine out of the 28 patients underwent weekly MRI scans during treatment for up to 7 weeks. The tumor sizes ranged from 0.28cc to 264.37 cc with average of 50.87 $\pm$55.89 cc. Respiratory triggered two-dimensional axial T2W turbo spin-echo sequence MRIs were acquired using a 16-element phased array anterior coil and a 44-element posterior coil and the following scan parameters: TR/TE = 3000-6000/120 ms, slice thickness = 2.5 mm and in-plane resolution of 1.1 $\times$ 0.97 mm$^2$ flip angle = 90°, number of slices = 43, number of signal averages = 2, and field of view = 300 $\times$ 222 $\times$ 150 mm$^3$.

### C. MRI abdomen dataset

Twenty T1-DUAL in-phase MRI and T2-weighted spectral pre-saturation inversion recovery (SPIR) sequence from the ISBI grand challenge Combined Healthy Abdominal Organ Segmentation (CHAOS) was analyzed. Image sets were acquired using a 1.5T Philips MRI, with an image resolution of 256 $\times$ 256 pixels, slice thickness that ranged between 5.5mm to 9mm (average of 7.84mm), x-y spacing that ranged between 1.36 - 1.89 mm (average 1.61 mm) and the number of slices that ranged between 26 and 50 (average 36).

## II. SEGMENTATION EVALUATION METRICS

The following metrics are used for segmentation evaluation.

- **Dice similarity coefficient (DSC)** was computed by comparing the algorithm and expert-segmentation as:

$$DSC = \frac{2 \times TP}{FP + 2 \times TP + FN} \tag{1}$$

where, TP is the number of true positives, FP is the number of false positives and FN is the number of false negatives.

- **Surface DSC** is computed using the DSC of the segmented and manually labelled surface, as shown in equation 2.

$$D_{i,j}^{(\tau)} = \frac{\mid S_i \cap B_j^{(\tau)} \mid + \mid S_j \cap B_i^{(\tau)} \mid}{\mid S_i \mid + \mid S_j \mid} \tag{2}$$

Where $B_i^{(\tau)} \subset R^3$ is a border region for the surface $S_i$. We calculate the surface dice with the tolerance $\tau$ of 2 $mm$.

- **The Hausdorff distance** was computed as:

$$Hausd(P,T) = max \left\{ \underset{p \in S_P}{sup}\, \underset{t \in S_t}{inf}\, (p,t) \, , \, \underset{t \in S_T}{sup}\, \underset{p \in S_P}{inf}\, (t,p) \right\}$$

where, P and T are ground truth and segmented volumes, and p,t are points on P and T, respectively. $S_p$ and $S_t$ correspond to the surface of P and T, respectively. To remove the influence of noise during evaluation, we used Hausdorff Distance (95%) as recommended by Menze.

## III. IMAGE SYNTHETIC EVALUATION METRICS

### A. KL divergence

The similarity of pseudo MRI to the T2w MRI was evaluated using Kullback–Leibler divergence(K-L divergence), as done previously [39], and quantifies the average statistical differences in the intensity distributions. The K-L divergence was computed using the intensity values within the tumor regions by comparing the intensity histogram for all the generated pseudo MR images and the intensity histogram computed from the training T2w MR images. The KL divergence measure quantifies the similarity in the overall intensity variations between the pseudo MR and the real MR images within the structure of interest, namely, tumors. The K-L divergence is calculated by equation 5:

$$D_{LK}(P_{sMRI}||Q(rMRI)) = \sum P_{sMRI} \ln \frac{P_{sMRI}}{Q_{rMRI}} \tag{3}$$

where $P_{sMRI}$ and $Q_{rMRI}$ indicate the tumor distribution in pseudo MR and T2w MR images and the summation is computed over a fixed number of discretized intensity levels (N = 1000).

### B. PSNR

The Peak signal-to-noise ratio (PSNR) is computed based on the pseudo MRI and real MRI using the following equation:

$$\text{PSNR} = 20\log_{10}(\frac{x_{max}}{RMSE}), x_{max} = \max(x_m) \tag{4}$$

where RMSE= $\frac{\sum_{m=1}^{M}(\hat{x}_m - x_m)^2}{M}$; $\hat{x}$ and $x_m$ represent the $m^{th}$ pixel values in the pseduo MRI and real MRI, respectively; $M$ is the number of pixels of one image; $x_{max}$ is the max valul of real MRI.

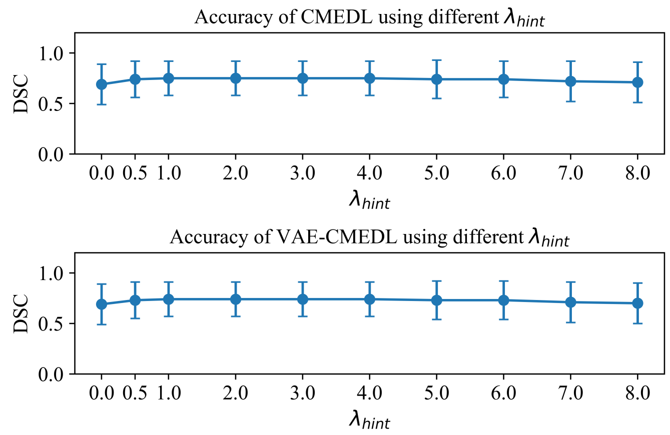


Fig. 1. Dice similarity coefficient segmentation accuracy for the left and right parotid glands computed at different settings of $\lambda_{hint}$.

### C. SSIM

The structural similarity index measure (SSIM) is computed as

$$\text{SSIM} = \left(\frac{(2\mu_{\hat{x}}\mu_x + C_1)(2\sigma_{cov} + C_2)}{(\mu_{\hat{x}}^2 + \mu_x^2 + C_1)(\sigma_{\hat{x}}^2 + \sigma_x^2 + C_2)}\right), \tag{5}$$

where $\mu_{\hat{x}}$ and $\sigma_{\hat{x}}$ indicate the mean and standard deviation of the pseudo MRI; $\mu_x$ and $\sigma_x$ denote the mean and standard deviation of the real MRI; $\sigma_{cov}$ is the covariance of the pseudo MRI and the real MRI; $C_1$ and $C_2$ are the regularization constraints depends on the dynamic range of the image.

## IV. Network hyper-parameter optimization

In the cylegan based image translation, we used the default setting of 10 for $\lambda_{cyc}$ and $\lambda_{cx}$=1 as done in [49, 51]. In the DRIT-VAE based image translation, we set $L_c = 1$, $\lambda_{vae} = 1$, $\lambda_{cc} = 10$, $\lambda_{lr} = 10$ as the default setting in [21]. The value of $\lambda_{seg}$ was set to 5 as done in our prior work applied to cross-modality lung tumor segmentation [39]. We computed the best setting for $\lambda_{hint}$ by evaluating a range of values consisting of [0.0,0.5,1,2,3,4,5,6,7,8]. Evaluation was done on the CT lung tumor and the selected value was used in all other datasets. Fig. 1 shows the segmentation performance on the validation set computed for lung tumor. As seen, the best performance was reached at a value of $\lambda_{hint} = 1$, beyond which the performance stabilized and began to drop beyond $\lambda_{hint} = 7$. Hence, this value of 1 was selected in all the experiments.

We chose a batch size of 1 because that was the largest number we could use given the memory and computational constraints. Also all the other networks used in the comparison experiments were trained with the same batch size and learning rates. Hence, additional hyper-parameter optimization of these parameters was not done for our approach.

## V. Additional cases for inter-rater segmentation

Fig. 2 shows two additional cases for inter-rater evaluation.

## VI. Computing resources

Computing resources of different networks is shown in Table VI. Training (ms) is computed as one single iteration using 256×256 image during training. Test (ms) is computed as a single image of size 256×256 inference time. Hardware information is shown below: NVIDIA V100 GPU (16Gb), CUDA 10.1, cudnn 7.0, Intel(R) Xeon(R) CPU E5-2697 v4 @ 2.30GHz.

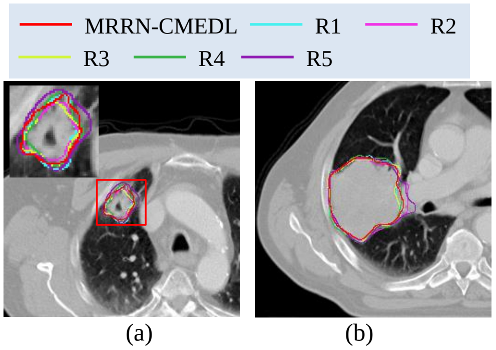


Fig. 2. CMEDL-MRRN segmentation (red) and five radiation oncoloigsts segmentation for representative tumors. Additional two cases for the inter-rater segmentation analysis.

TABLE I
Computing requirements for different segmentation methods.

| NetWork | Method | Param(M) | Train(ms) | Test(ms) | Test GPU | GFLOPs |
|---|---|---|---|---|---|---|
| | CT only | 13.39 | 130 | | | 30.98 |
| Unet | VAE-CMEDL | 81.39 | 1560 | 8.1 | 1.45G | 135.23 |
| | CMEDL | 41.65 | 464 | | | 160.92 |
| | CT only | 1.37 | 136 | | | 11.34 |
| DenseFCN | VAE-CMEDL | 69.37 | 1520 | 11.7 | 2.17G | 84.88 |
| | CMEDL | 29.63 | 759 | | | 121.64 |
| | CT only | 38.92 | 390 | | | 41.36 |
| MRRN | VAE-CMEDL | 106.92 | 2253 | 17.8 | 2.21G | 156.26 |
| | CMEDL | 67.18 | 869 | | | 181.68 |

## VII. Additional Feature map visualization

Fig. 3 shows addtional case of visualization of feature maps in the channels one to twenty four of the last layer(with size of 256×256×64) for a standard Unet (Fig. 3(a)), CMEDL Unet teacher network (Fig. 3(b)), and the CMEDL CT student network (Fig. 3(c)). As shown, the feature maps for the student network match the teacher network's activations very closely and better differentiate the tumor from its background compared to the CT only network.

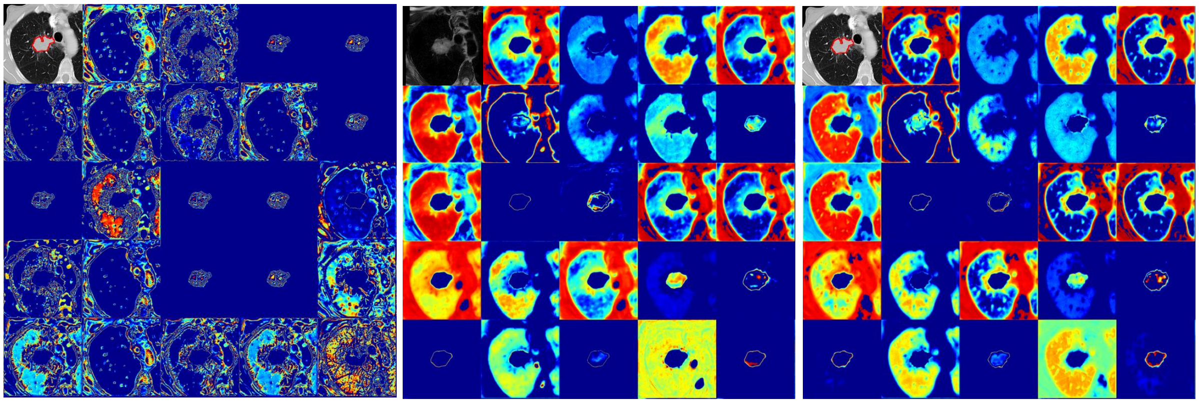


Fig. 3. The 1-24 channel feature maps from last layer of the model trained using (a) only CT images and proposed (b) CMEDL-MRI and (c) CMEDL-CT. The tumor region is enclosed in the red contour.
